# Supplementary material for: ALAS: Transactional and Dynamic Multi-Agent LLM Planning
Source: arXiv:2511.03094 source file (2025-11-05)
Supplement: Supplementary file 1 [file AppendixImplementationSpec.tex]

\section{ALAS Implementation Specification}
\label{app:implementation-spec}

The hybrid $\MP$ architecture enables the integration of Claude's meta-planning capabilities with local execution systems through a layered approach. The three-layer architecture, comprising local control, integration and planning layer interfaces, handles different aspects of $\MP$ execution through well-defined interfaces. The meta-planner $\MP$ algorithm resides in the Integration Layer, where it efficiently coordinates between Claude's planning capabilities and local execution. This placement allows the MP to maintain oversight while minimizing communication overhead.

Problem specifications and constraints are uploaded through the Planning Layer interface to Claude, which performs initial problem analysis and formulation. Claude then collaborates with $\mathcal{MP}$ in the Integration Layer to develop the execution strategy. This interaction occurs through standardized JSON protocols that maintain consistency between planning decisions and execution requirements.

Agent specifications and implementations reside in the Local Control Layer, where they are directly accessible for execution. However, their orchestration is managed by the MP in the Integration Layer. This separation enables rapid local responses while maintaining global coordination. Agents communicate with $\mathcal{MP}$ through event-driven protocols, using WebSocket connections for real-time updates and REST APIs for state synchronization.

When conditions require replanning, the Local Control Layer signals the Integration Layer through its event system. The MP evaluates the situation and, when necessary, initiates consultation with Claude through the Planning Layer. This multi-level response system facilitates both rapid local adaptations and thoughtful strategic replanning.

\begin{figure}[ht]
\centering
\begin{tikzpicture}[node distance=2cm]
   % Define the layers as rectangles
   \draw[fill=blue!10] (0,0) rectangle (5,2) node[pos=.4] {Local Control Layer};
   \draw[fill=cyan!20] (0,2.5) rectangle (5,4.5) node[pos=.4] {Integration Layer};
   \draw[fill=blue!10] (0,5) rectangle (5,7) node[pos=.4] {Planning Layer (Claude)};
   
   % Add arrows showing data flow
   \draw[-latex] (3,2) -- (3,2.5);
   \draw[-latex] (3.5,2.5) -- (3.5,2);
   \draw[-latex] (3,4.5) -- (3,5);
   \draw[-latex] (3.5,5) -- (3.5,4.5);
   
   % Add labels for arrows
   \node[rotate=90] at (2.7,2.25) {\small State Updates};
   \node[rotate=90] at (3.8,2.25) {\small Commands};
   \node[rotate=90] at (2.7,4.75) {\small Queries};
   \node[rotate=90] at (3.8,4.75) {\small Plans};
\end{tikzpicture}
\caption{Hybrid $\MP$ Architecture}
\label{fig:hybrid-arch}
\end{figure}

The architecture's three layers
are specified below.

\subsection{Local Control Layer}
\begin{itemize}[leftmargin=1em, topsep=-.1pt, itemsep=-.1pt, label=*]
   \item State Management Database
       \begin{itemize}[leftmargin=1em, topsep=-.1pt, itemsep=-.1pt, label=-]
           \item PostgreSQL with TimescaleDB extension
           \item Real-time GPS coordinates (5Hz update)
           \item Vehicle telemetry and status
           \item Task execution states
       \end{itemize}
   \item Safety Monitor
       \begin{itemize}[leftmargin=1em, topsep=-.1pt, itemsep=-.1pt, label=-]
           \item Constraint violation detection
           \item Emergency response protocols
           \item Heartbeat monitoring (100ms)
       \end{itemize}
\end{itemize}

\subsection{Integration Layer}
\begin{itemize}[leftmargin=1em, topsep=-.1pt, itemsep=-.1pt, label=*]
   \item Communication Protocol
       \begin{itemize}[leftmargin=1em, topsep=-.1pt, itemsep=-.1pt, label=-]
           \item REST API with WebSocket support
           \item JSON state representation schema
           \item Binary protocol for sensor data
       \end{itemize}
   \item State Synchronization
       \begin{itemize}[leftmargin=1em, topsep=-.1pt, itemsep=-.1pt, label=-]
           \item Event-driven updates
           \item Conflict resolution logic
           \item Version control for state updates
       \end{itemize}
\end{itemize}

\subsection{Planning Layer Interface}
\begin{itemize}[leftmargin=1em, topsep=-.1pt, itemsep=-.1pt, label=*]
   \item Claude API Integration
       \begin{itemize}[leftmargin=1em, topsep=-.1pt, itemsep=-.1pt, label=-]
           \item Authentication handling
           \item Request rate limiting
           \item Response parsing and validation
       \end{itemize}
   \item Query Formation
       \begin{itemize}[leftmargin=1em, topsep=-.1pt, itemsep=-.1pt, label=-]
           \item State compression algorithms
           \item Priority-based scheduling
           \item Context window management
       \end{itemize}
\end{itemize}

\subsection{Performance Requirements}
\begin{itemize}[leftmargin=1em, topsep=-.1pt, itemsep=-.1pt, label=*]
   \item Local operations: < 500ms latency
   \item State synchronization: < 100ms
   \item Claude consultation: < 2s end-to-end
   \item System state consistency: 99.9\%
   \item Minimum 99.99\% uptime for local components
\end{itemize}
