# Supplementary material for: ALAS: Transactional and Dynamic Multi-Agent LLM Planning
Source: arXiv:2511.03094 source file (2025-11-05)
Supplement: Supplementary file 2 [file AppendixValidationRefinement.tex]

\section{Phase Validation and Refinement}
\label{app:vlidation-spec}
